# Supplementary material for: A Compact Dynamic 3D Gaussian Representation for Real-Time Dynamic View Synthesis
Source: arXiv:2311.12897 source file (2024-07-04)
Supplement: Supplementary file 1 [file X_suppl.tex]

{
        \centering
        \Large
        \vspace{0.5em}Supplementary Material \\
        \vspace{1.0em}
   }

\section{Additional Qualitative Results}
We can divide training inputs into subsets to improve rendering quality. \Cref{fig:short} shows the rendering results trained on first 60 frames and all 300 frames.
In exchange for the gains in rendering quality, the models trained on 60 frames require extra memory size for the whole scene. 
The memory size is around 1.9GB and it is still three times smaller than storing Guassians parameters per timestep. The result shows our method can control the reconstruction quality by
dividing frames.
\Cref{fig:hypernerf_interp,fig:hypernerf_misc}  show further novel view synthesis results of our method, demonstrating that our method can reconstruct a wide range of scenes.

\begin{figure}[t]
  \centering
  \bgroup 
   
  \setlength\tabcolsep{0.2pt}
  \begin{tabular}{cc}
    300 frames & 60 frames \\\\
    \includegraphics[width=0.45\linewidth]{supp/00014.png} &
    \includegraphics[width=0.45\linewidth]{supp/short00014.png} 
  \end{tabular}\egroup
\caption{Reducing training frames improves rendering quality while increasing memory size. The moemory size is still compact. }\label{fig:short}
\end{figure}

\begin{figure}[t]
  \centering
  \bgroup 
   
  \setlength\tabcolsep{0.2pt}
  \begin{tabular}{cccc}
    Ground Truth & Ours &     Ground Truth & Ours \\\\
\includegraphics[width=0.25\linewidth]{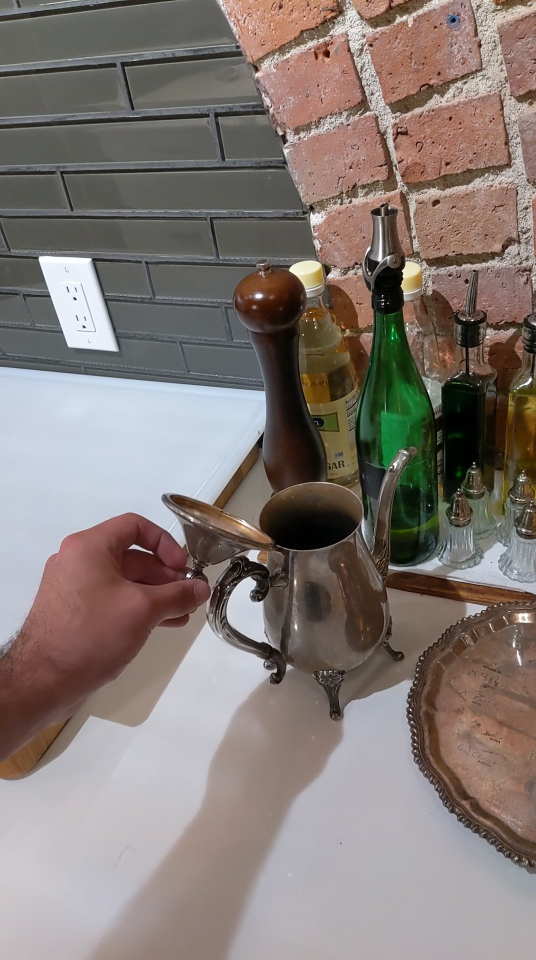} &
\includegraphics[width=0.25\linewidth]{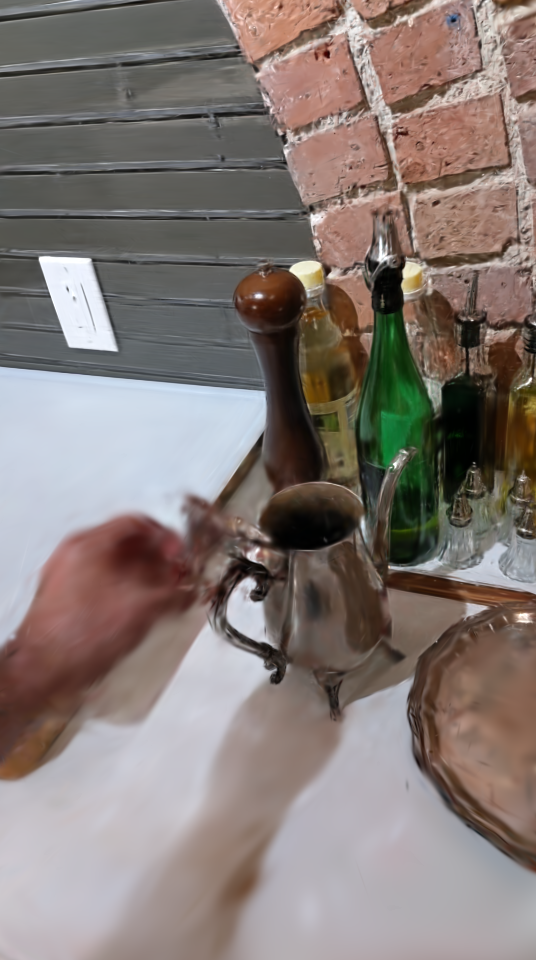} &
\includegraphics[width=0.25\linewidth]{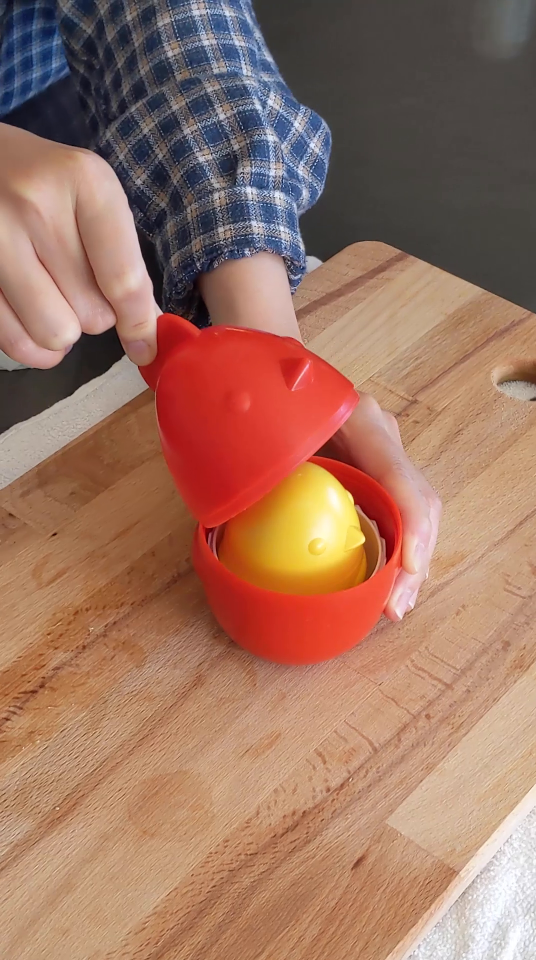} &
\includegraphics[width=0.25\linewidth]{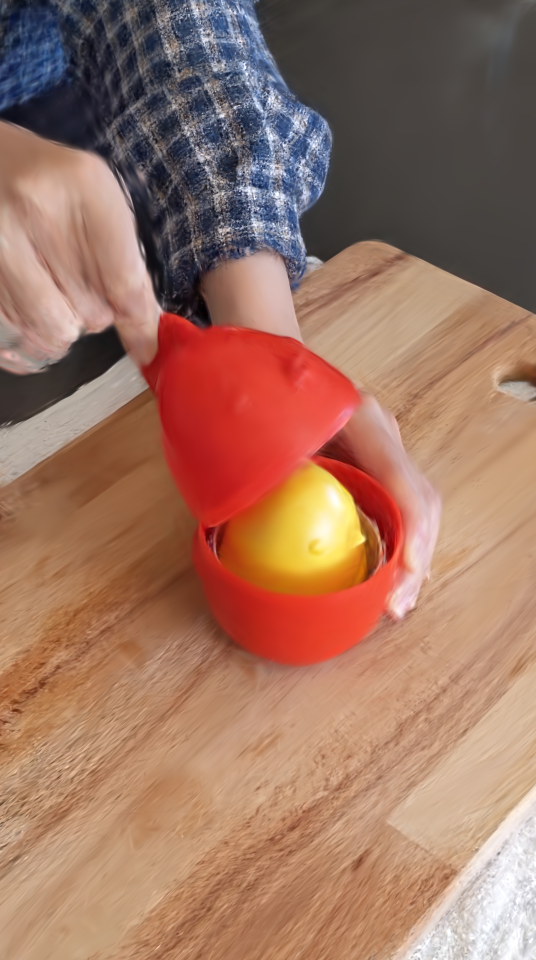} \\
    Ground Truth & Ours &     Ground Truth & Ours \\\\
\includegraphics[width=0.25\linewidth]{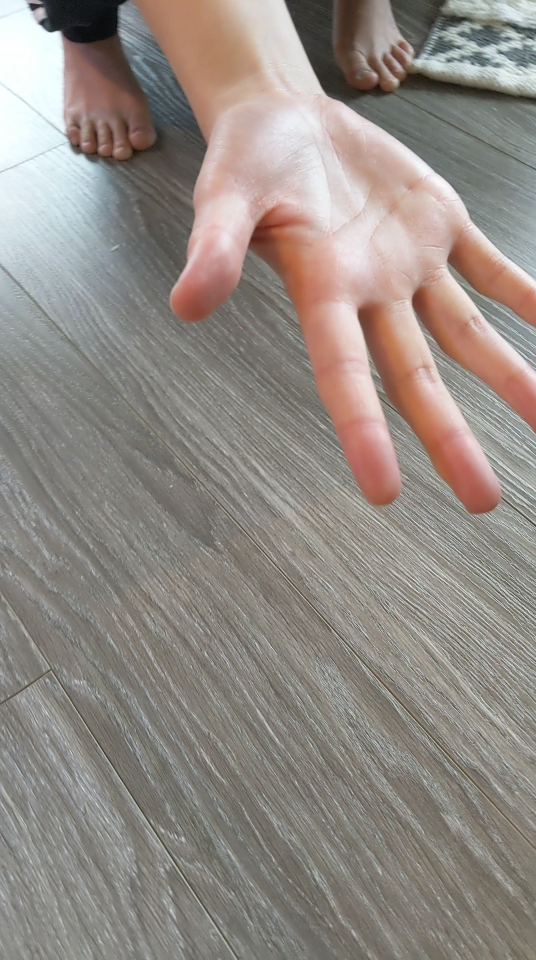} &
\includegraphics[width=0.25\linewidth]{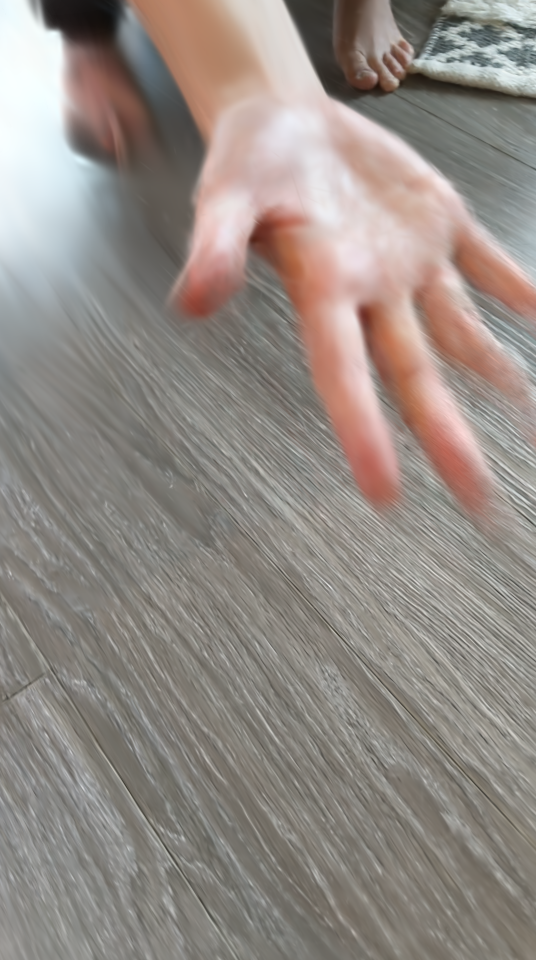} &
\includegraphics[width=0.25\linewidth]{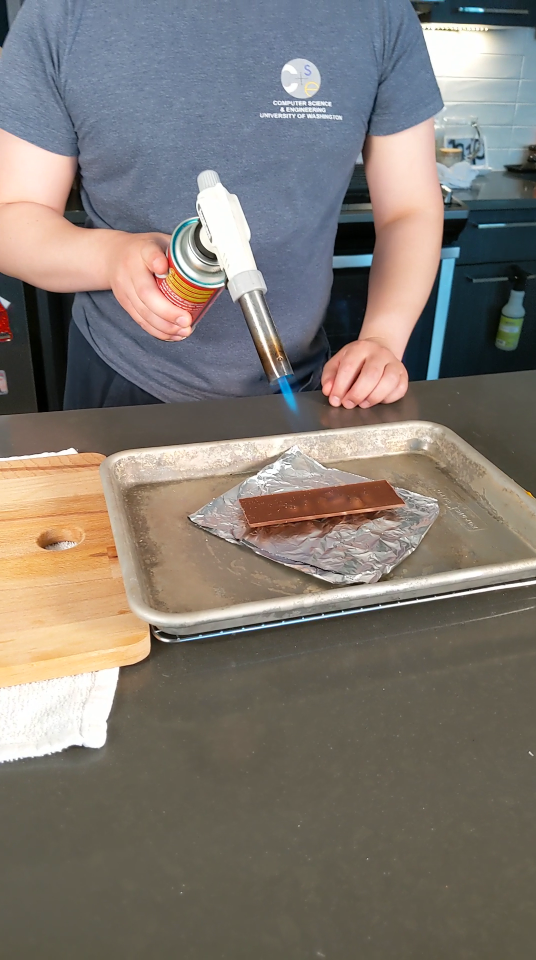} &
\includegraphics[width=0.25\linewidth]{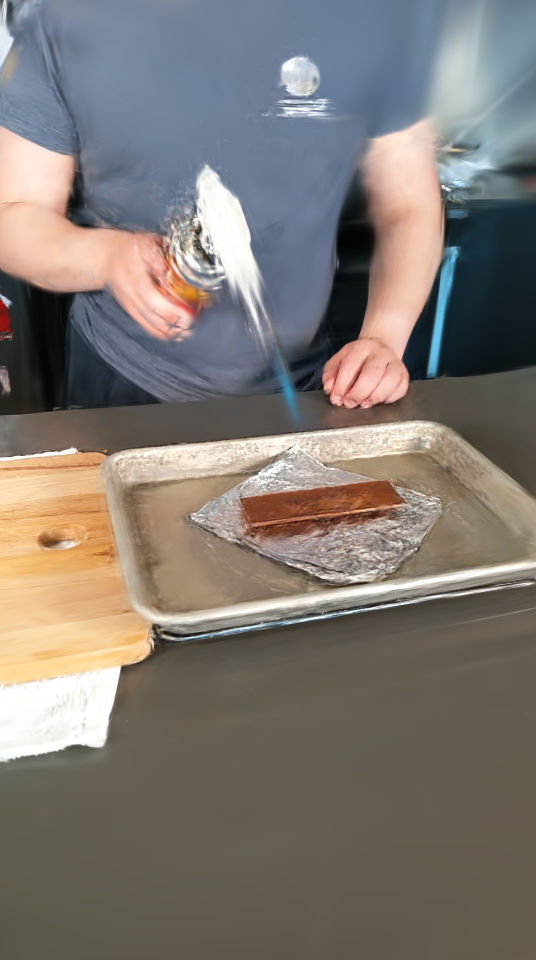} \\
  \end{tabular}
  \begin{tabular}{cc}
    Ground Truth & Ours    \\
\includegraphics[width=0.5\linewidth]{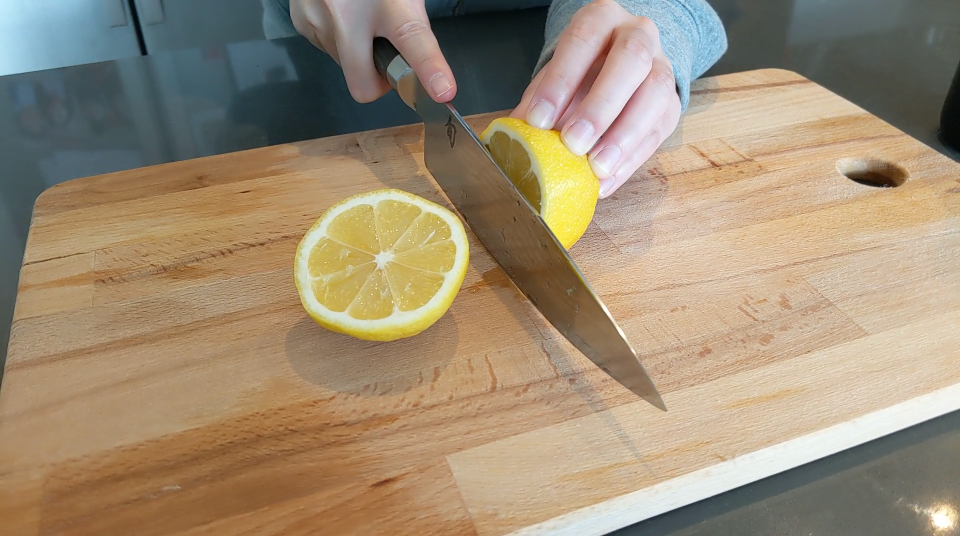} &
\includegraphics[width=0.5\linewidth]{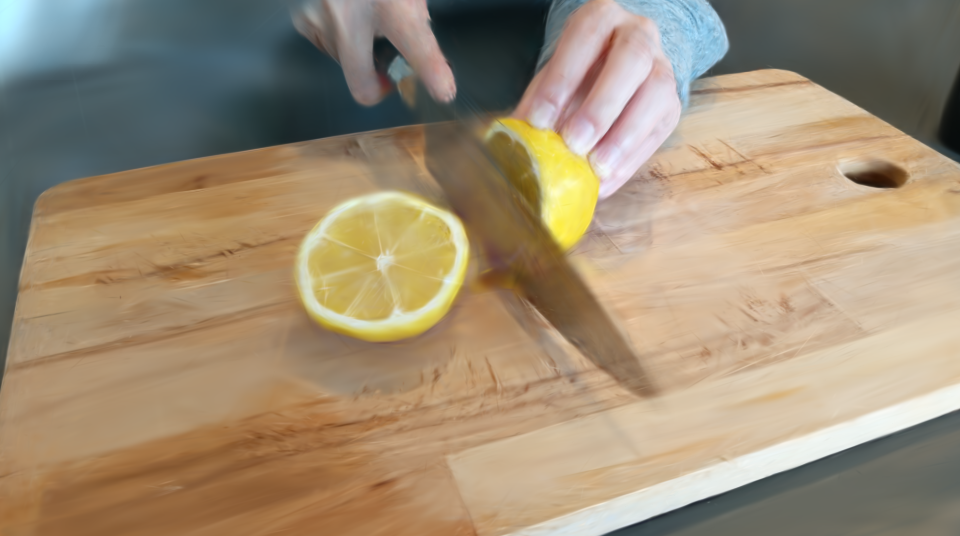} \\
  \end{tabular}  \egroup
\caption{Qualitative examples on HyperNeRF~\cite{park2021hypernerf}. Visual quality of our method depends on the complexity of target scenes.}\label{fig:hypernerf_interp}
\end{figure}

\begin{figure*}[t]
  \centering
  \bgroup 
   
  \setlength\tabcolsep{0.2pt}
  \begin{tabular}{cccc}
    Ground Truth & Ours & Ground Truth & Ours \\\\
\includegraphics[width=0.18\linewidth]{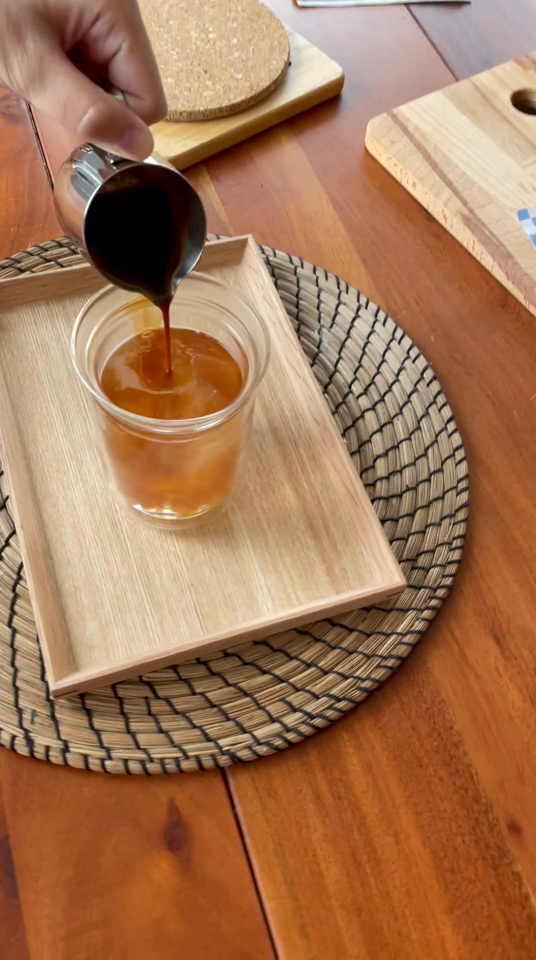} &
\includegraphics[width=0.18\linewidth]{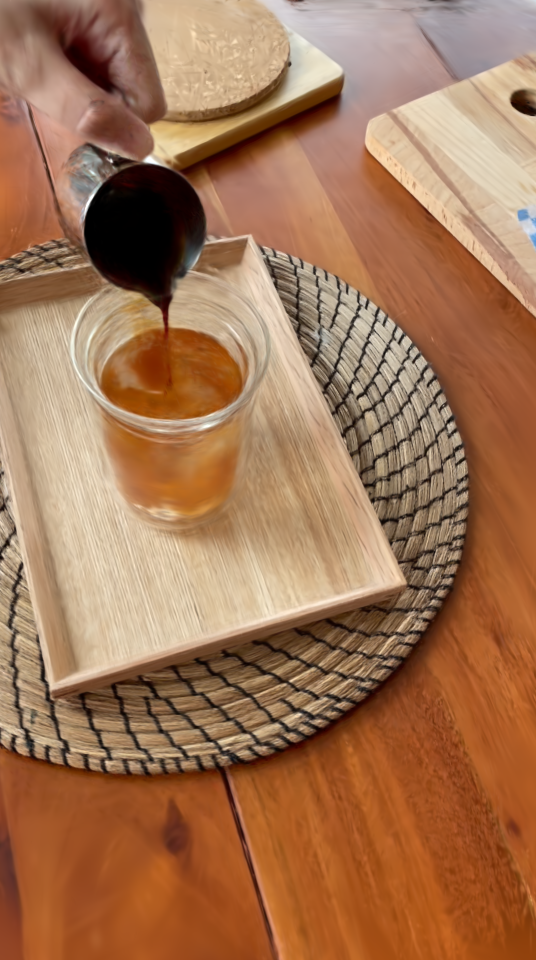} &
\includegraphics[width=0.18\linewidth]{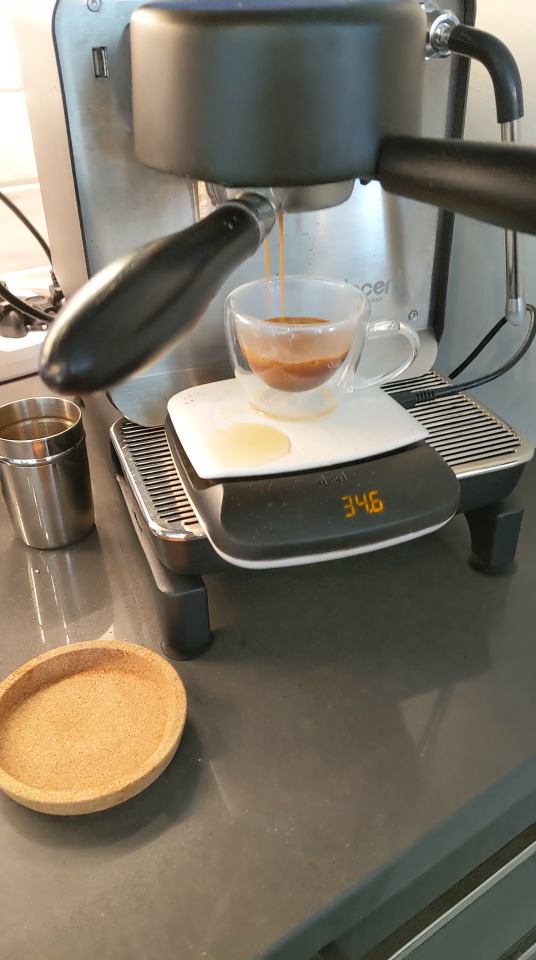} &
\includegraphics[width=0.18\linewidth]{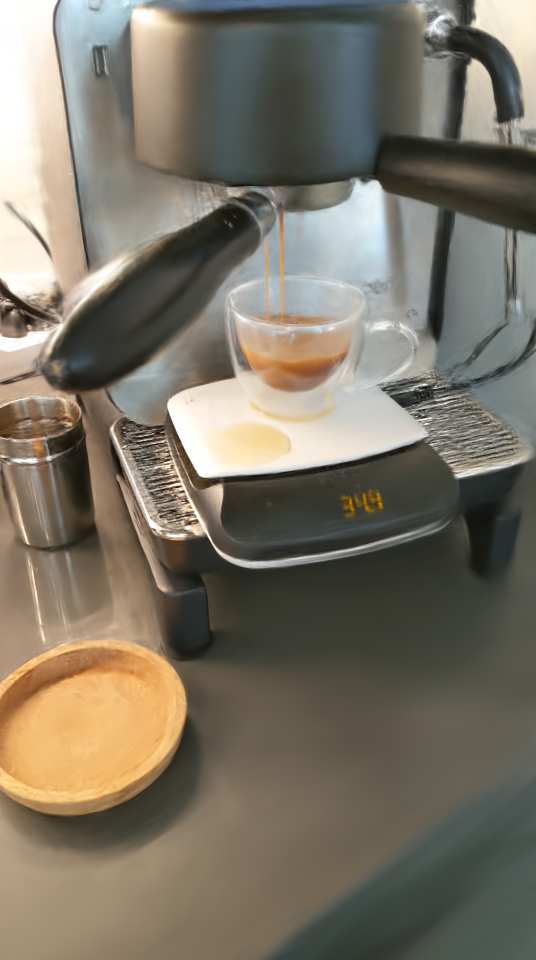} \\
\includegraphics[width=0.18\linewidth]{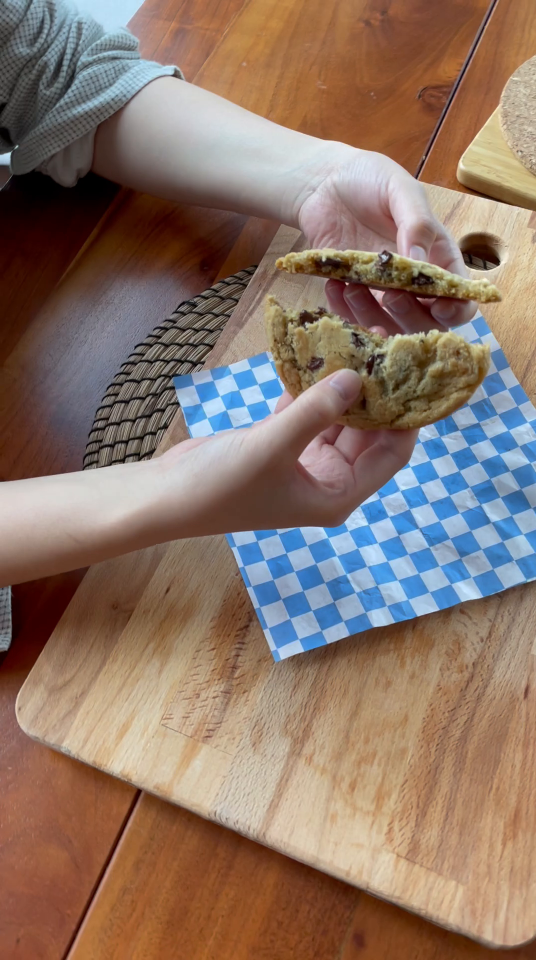} &
\includegraphics[width=0.18\linewidth]{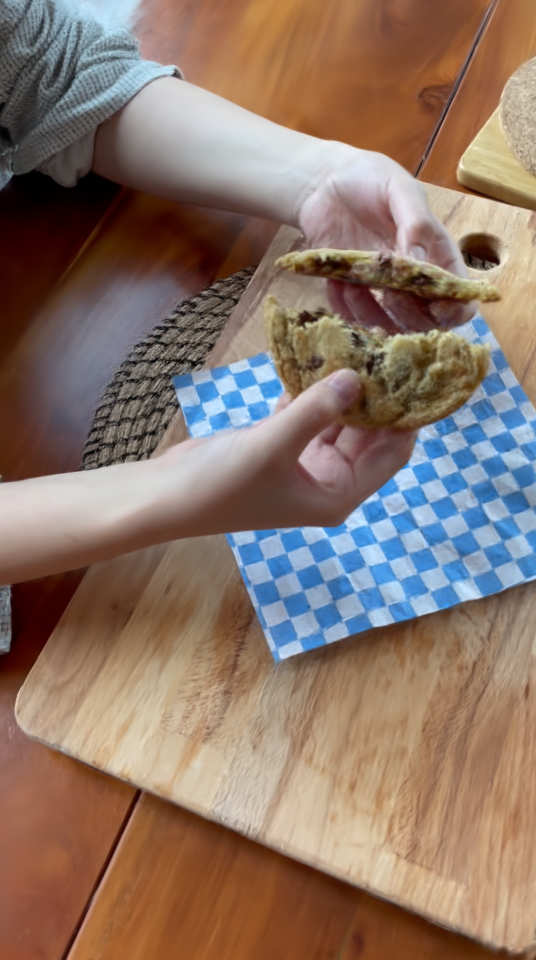} &
\includegraphics[width=0.18\linewidth]{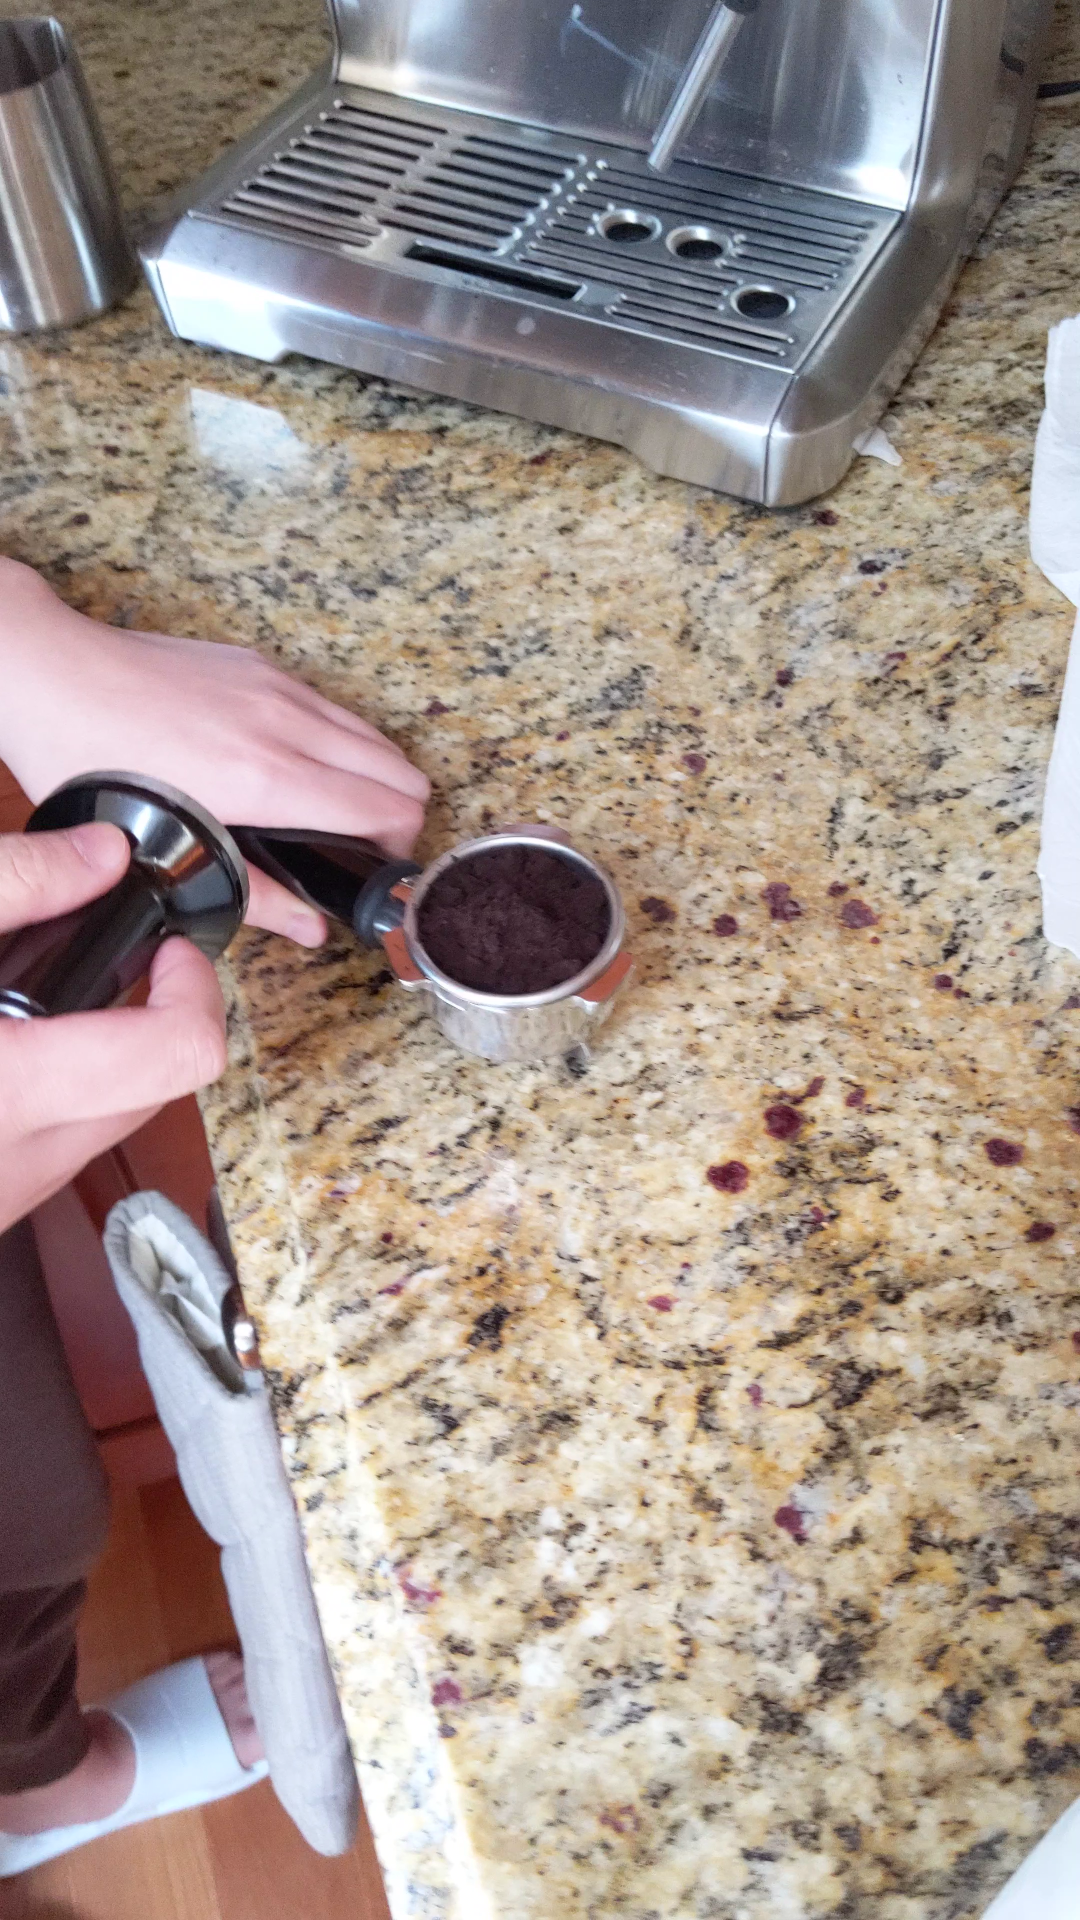} &
\includegraphics[width=0.18\linewidth]{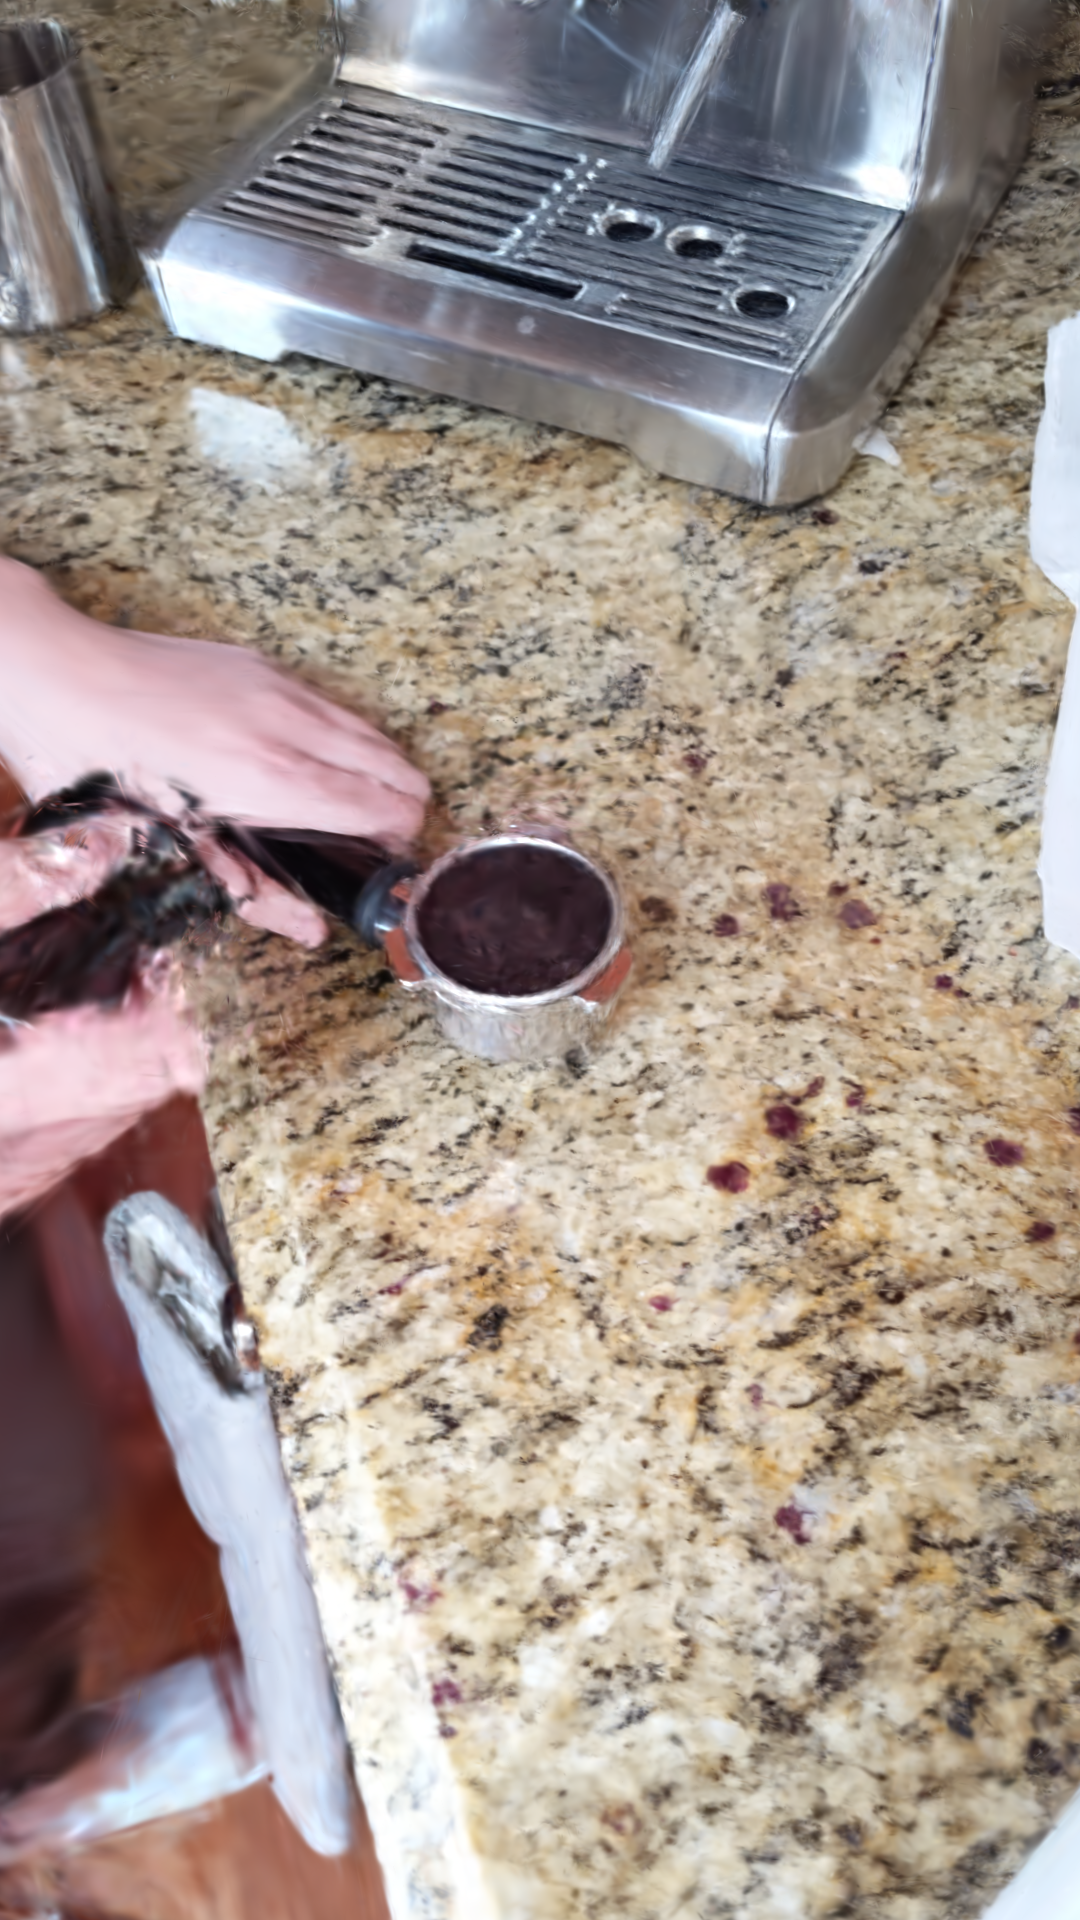} \\
  \end{tabular}
  \begin{tabular}{cc}
\includegraphics[width=0.33\linewidth]{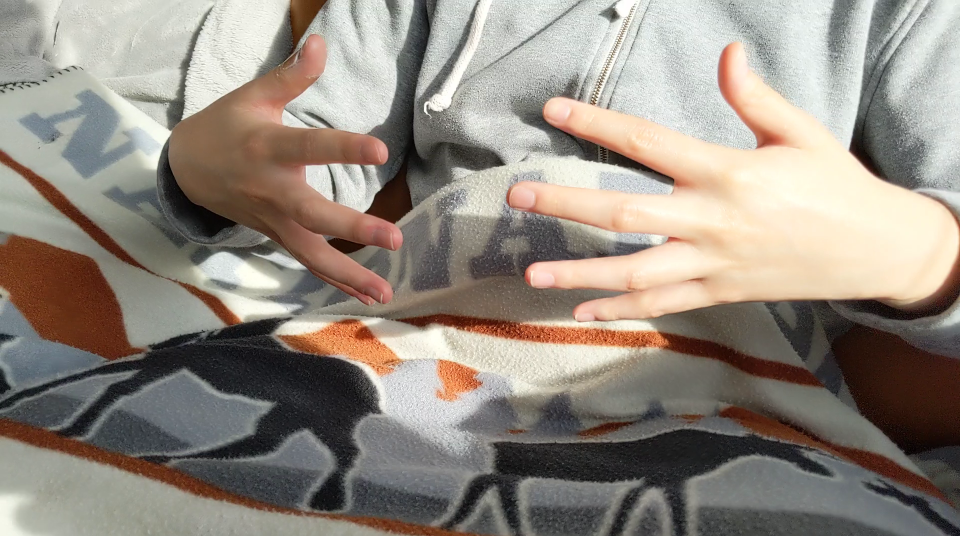} &
\includegraphics[width=0.33\linewidth]{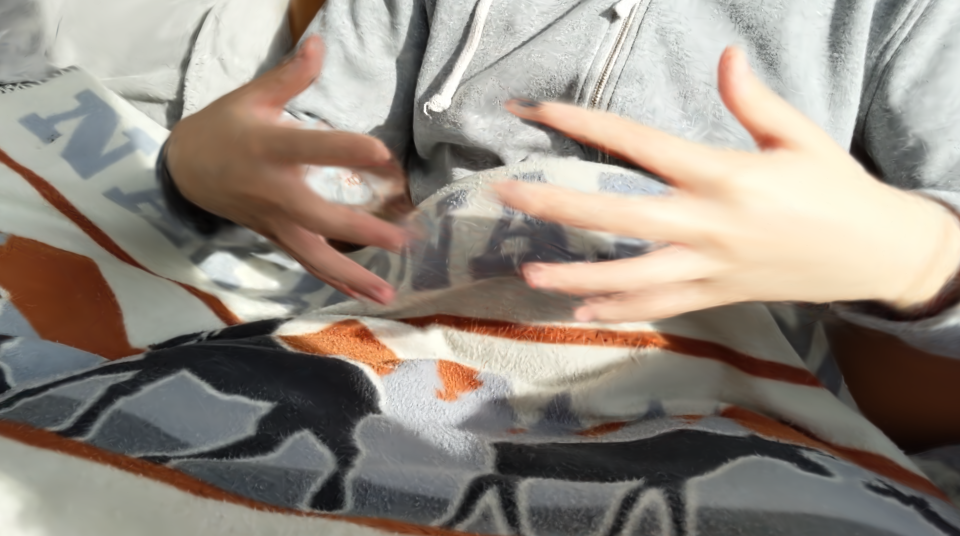} \\
\includegraphics[width=0.33\linewidth]{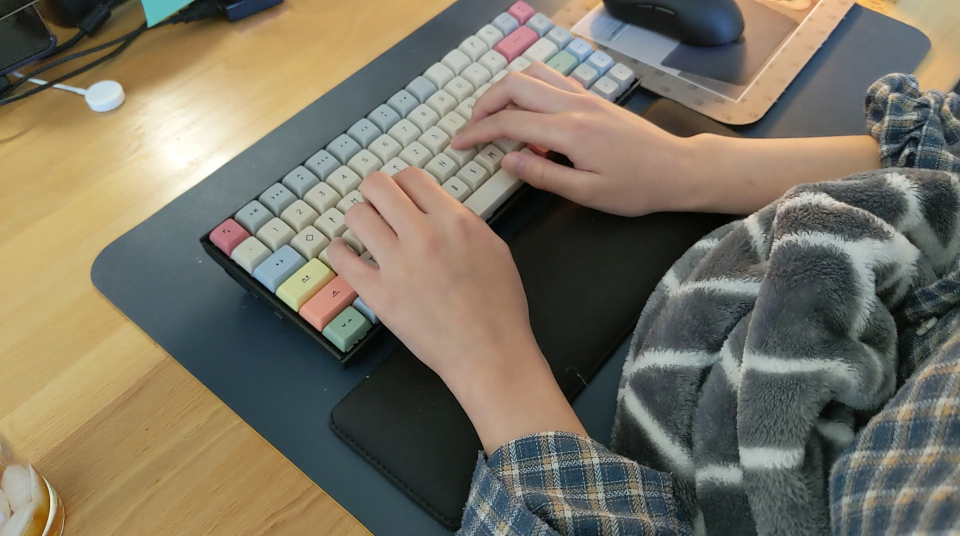} &
\includegraphics[width=0.33\linewidth]{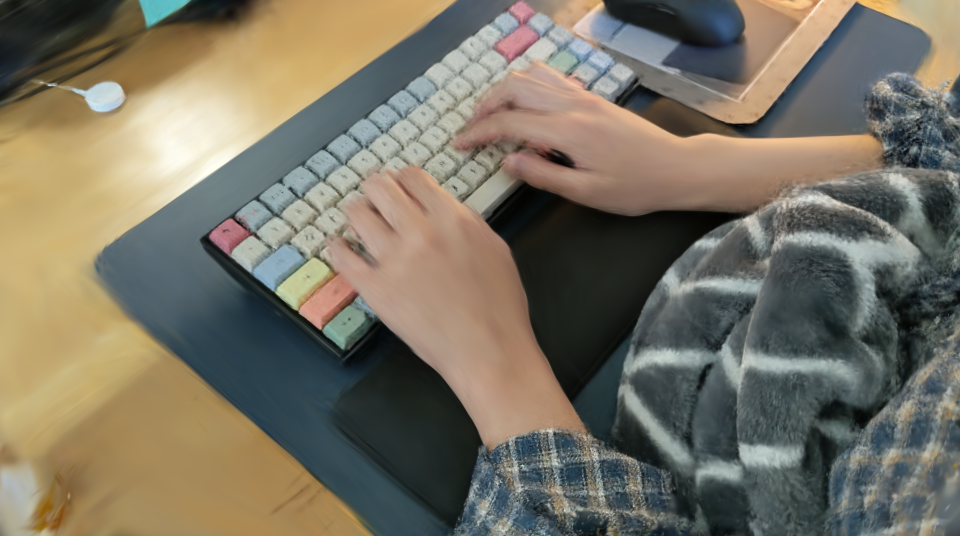} \\
  \end{tabular}\egroup
\caption{Qualitative examples on HyperNeRF~\cite{park2021hypernerf}. Our method reconstruct scenes faithfully and struggle to model complex motions.}\label{fig:hypernerf_misc}
\end{figure*}

\section{Additional Quantitative Results}
We show the ablation study of the flow loss ($\loss_{\rm flow}$) in \cref{tb:flow}. 
The flow loss improves visual quality of some scenes out of benchmark scenes.
We also investigate the effects of the number of harmonics in Fourier approximation $L$ in \cref{tb:dynerf_l}.
The method is robust to the hyperparameter except when $L$ is extremely small ($L=1,2$).

\begin{table*}[tb]
\caption{Effects of flow reconstruction. The flow reconstruction enhance the performance of some cases and the average scores.}\label{tb:flow}
\resizebox{\linewidth}{!}{
\begin{tabular}{ccccccccccccccc}\toprule
& \multicolumn{2}{c}{\textsc{Sear Steak}} &
\multicolumn{2}{c}{\textsc{Cut Roasted Beef}} &
\multicolumn{2}{c}{\textsc{Cook Spinach}} &
\multicolumn{2}{c}{\textsc{Coffee Martini}} &
\multicolumn{2}{c}{\textsc{Flame Salmon 1}} &
\multicolumn{2}{c}{\textsc{Flame Steak}} & \multicolumn{2}{c}{\textbf{Mean}}\\\cmidrule(l{2pt}r{2pt}){2-3}\cmidrule(l{2pt}r{2pt}){4-5}\cmidrule(l{2pt}r{2pt}){6-7} \cmidrule(l{2pt}r{2pt}){8-9} \cmidrule(l{2pt}r{2pt}){10-11} \cmidrule(l{2pt}r{2pt}){12-13} \cmidrule(l{2pt}r{2pt}){14-15}
& PSNR$\uparrow$ & SSIM$\uparrow$  & PSNR$\uparrow$ & SSIM$\uparrow$ & PSNR$\uparrow$ & SSIM$\uparrow$ & PSNR$\uparrow$ & SSIM$\uparrow$ & PSNR$\uparrow$ & SSIM$\uparrow$ & PSNR$\uparrow$ & SSIM$\uparrow$ & PSNR$\uparrow$ & SSIM$\uparrow$ \\\midrule
Ours w/o flow & 29.4 & 0.969 & 32.5 & \best{0.970} & 31.2 & 0.964 & 25.5 & 0.916 & 25.8 & 0.909 & 28.4 & 0.965 & 28.8 & 0.948\\
Ours & \best{33.1} & \best{0.976} & \best{32.7} & 0.969 &\best{ 31.8} & \best{0.966} & \best{26.1} & \best{0.922}  & \best{26.0} & \best{0.926} & \best{33.1} & \best{0.974} & \best{30.4} & \best{0.955} \\\bottomrule
\end{tabular}}
\end{table*}

\begin{table}[tb]
\caption{Per scene results on different $L$. The results on $L=5$ achieve better trade-offs between performance and complexity (model size).}\label{tb:dynerf_l}
\resizebox{\linewidth}{!}{
\begin{tabular}{ccccccccccccccc}\toprule
& \multicolumn{2}{c}{\textsc{Sear Steak}} &
\multicolumn{2}{c}{\textsc{Cut Roasted Beef}} &
\multicolumn{2}{c}{\textsc{Cook Spinach}} &
\multicolumn{2}{c}{\textsc{Coffee Martini}} &
\multicolumn{2}{c}{\textsc{Flame Salmon 1}} &
\multicolumn{2}{c}{\textsc{Flame Steak}} & \multicolumn{2}{c}{\textbf{Mean}}\\\cmidrule(l{2pt}r{2pt}){2-3}\cmidrule(l{2pt}r{2pt}){4-5}\cmidrule(l{2pt}r{2pt}){6-7} \cmidrule(l{2pt}r{2pt}){8-9} \cmidrule(l{2pt}r{2pt}){10-11} \cmidrule(l{2pt}r{2pt}){12-13} \cmidrule(l{2pt}r{2pt}){14-15}
& PSNR$\uparrow$ & SSIM$\uparrow$  & PSNR$\uparrow$ & SSIM$\uparrow$ & PSNR$\uparrow$ & SSIM$\uparrow$ & PSNR$\uparrow$ & SSIM$\uparrow$ & PSNR$\uparrow$ & SSIM$\uparrow$ & PSNR$\uparrow$ & SSIM$\uparrow$ & PSNR$\uparrow$ & SSIM$\uparrow$ \\\midrule
$L=1$ & 25.9 & 0.944 & 30.0 & 0.952 & 30.2 & 0.953 & 25.8 & 0.917 & 25.4 & 0.922 & 27.5 & 0.944 & 27.5 & 0.938\\
$L=2$ & 29.5 & 0.965 & 24.2 & 0.923 & 30.7 & 0.957 & 25.8 & 0.919 & 24.4 & 0.910 & 24.5 & 0.932 & 26.5 & 0.934\\
$L=3$ & 32.3 & 0.974 & 31.9 & 0.965 & 31.4 & 0.962 & 26.1 & 0.923 & 25.8 & 0.924 & 30.1 & 0.967 & 29.6 & 0.952\\
$L=4$ & 33.1 & 0.976 & 22.3 & 0.909 & 31.5 & 0.964 & 26.1 & 0.924 & 26.2 & 0.931 & 29.3 & 0.969 & 28.1 & 0.945\\
$L=5$ & 33.1 & 0.976 & 32.7 & 0.969 & 31.8 & 0.966 & 26.1 & 0.922 & 26.0 & 0.926 & 33.1 & 0.974 & 30.4 & 0.955\\
$L=6$ & 31.9 & 0.975 & 32.6 & 0.970 & 31.9 & 0.966 & 26.0 & 0.920 & 26.4 & 0.930 & 31.4 & 0.972 & 30.0 & 0.955\\
$L=7$ & 33.3 & 0.977 & 31.1 & 0.967 & 32.0 & 0.967 & 26.2 & 0.923 & 26.4 & 0.929 & 30.4 & 0.969 & 29.9 & 0.955\\
$L=8$ & 31.9 & 0.975 & 32.8 & 0.970 & 32.0 & 0.966 & 26.2 & 0.920 & 26.1 & 0.928 & 30.8 & 0.972 & 30.0 & 0.955\\
\bottomrule
\end{tabular}}
\end{table}
